# Supplementary material for: Do Text Simplification Systems Preserve Meaning? A Human Evaluation via Reading Comprehension
Source: arXiv:2312.10126 source file (2024-02-28)
Supplement: Supplementary file 1 [file 6_appendix.tex]

\section{RC Question and Types}
\label{sec:rc_data}

\paragraph{Coverage}

\paragraph{Question Types}

\paragraph{Example Questions}
